# Supplementary material for: Towards Fairness of Cryptocurrency Payments
Source: arXiv:1609.07256 source file (2016-12-01)
Supplement: Supplementary file 1 [file appendix_bf.tex]

%!TEX root = ../submission.tex
\section*{Appendix A: Bloomfilter Algorithms}
\label{sec:appendBGAlgos}

\begin{algorithm}
\caption{Bloom filter search}
\label{algo:bfsearch}
\begin{algorithmic}
% \Function{process\_block}{$query\_data, block\_id$}
    \\

    \State $pos\_y_i \gets $ position of the first $y_i$ in the mapped block
    \State $pos\_y_{end} \gets $ position of the last $y_i$ in the mapped block
    
    \State $S^\prime$ subset of $S$, where $y_i \leq s_i \leq y_{end}$

    % \State $*ptr\_query\_rep \gets $ pointer to the query representation
    % \State $*ptr\_dummy \gets $ pointer to a dummy value
    \State $pos\_s_i \gets $ position of the first $s_i \in S^\prime$
    \State $ctr\_dummy$ // a dummy counter

    \\ 
    \While{$pos\_y_i < pos\_y_{end}$}
      \\
      \If {$pos\_s_i$ equals $ pos\_y_i$}
        \State $update s_i with y_i$
        \State $pos\_s_i \gets position of $ 
      \Else       
        \State $(*ptr\_dummy).value \gets y_i$
        \State $*ptr\_dummy++ $
      \EndIf
      \State $pos\_y_i \gets $ position of the next $y_i$ in the mapped block
      \\
            
    \EndWhile
    \\

% \EndFunction
\end{algorithmic}
\end{algorithm}

\begin{algorithm}
\caption{Cuckoo search}
\label{algo:cuckoo}
\begin{algorithmic}
   \\

    \State $pos\_y_i \gets $ position of the first $y_i$ in the mapped block
    \State $pos\_y_{end} \gets $ position of the last $y_i$ in the mapped block
    
    \State $*ptr\_query\_rep \gets $ pointer to the query representation
    \State $*ptr\_dummy \gets $ pointer to a dummy value
    
    \\ 
    \While{$pos\_y_i < pos\_y_{end}$}
      \\
      \If {$(*ptr\_query\_rep).pos$ equals $ pos\_y_i$}
        \State $(*ptr\_query\_rep).value \gets y_i$
        \State $*ptr\_query\_rep++ $
      \Else       
        \State $(*ptr\_dummy).value \gets y_i$
        \State $*ptr\_dummy++ $
      \EndIf
      \State $pos\_y_i \gets $ position of the next $y_i$ in the mapped block
      \\
            
    \EndWhile
    \\
\end{algorithmic}
\end{algorithm}

\begin{algorithm}
\caption{Sequence of differences}
\label{algo:sod}
\begin{algorithmic}
   \\

    \State $pos\_y_i \gets $ position of the first $y_i$ in the mapped block
    \State $pos\_y_{end} \gets $ position of the last $y_i$ in the mapped block
    
    \State $*ptr\_query\_rep \gets $ pointer to the query representation
    
    \\ 
    \While{$pos\_y_i < pos\_y_{end}$}
      \\
      \State $binary\_search(ptr\_query\_rep, y_i)$
      \State $pos\_y_i \gets $ position of the next $y_i$ in the mapped block
      \\
            
    \EndWhile
    \\
\end{algorithmic}
\end{algorithm}

\begin{algorithm}
\caption{Initialize}
\label{algo:init}
\begin{algorithmic}
\Function{initialize}{}
  \State /* add a dummy item in lookup link-list 
  \State  * with position value larger than bloom filter size.
  \State  * The item is never processed hence we avoid checking 
  \State  * next item in link-list is empty before moving to next item
  \State  * This optimization avoids checking for next item equals null 
  \State  * while updating link list after processing each byte in Algorithm~\ref{algo:bfsearch} */
  \\
  \State $pos \gets $ integer larger than bloom filter size
  \\
  
  \State add\_lookup\_items($pos$)
\EndFunction
\end{algorithmic}
\end{algorithm}

%%%%%%%%%%%%%%%%%%%%%%%%%%%%%%%%%%%%%%%%
\begin{algorithm}
\caption{Uninitialize}
\label{algo:uninit}
\begin{algorithmic}
\Function{uninitialize}{}
  
  \State // Remove remaining items in query link-list
  \State // Remove remaining items in lookup link-list
  
\EndFunction
\end{algorithmic}
\end{algorithm}

%%%%%%%%%%%%%%%%%%%%%%%%%%%%%%%%%%%%%%%%
\begin{algorithm}
\caption{Extracting queries from $query\_data$}
\label{algo:extractQuery}
\begin{algorithmic}
  \For{each $query$ in $query\_data$ }
    \State extract $query\_id$
    \State extract $query\_value$
    \State $add\_query(query\_id, query\_value, block\_id)$ \hskip3em //Algorithm~\ref{algo:addQuery}
  \EndFor

\end{algorithmic}
\end{algorithm}

%%%%%%%%%%%%%%%%%%%%%%%%%%%%%%%%%%%%%%%%
\begin{algorithm}
\caption{Adding queries to link-lists}
\label{algo:addQuery}
\begin{algorithmic}
\Function{add\_query}{$query, query\_id, block\_id$}
  
  \State $bf\_poss \gets bloomfilter\_poss(query, BF\_POSS) $
  \\

  \For{each bf\_poss[i]}
    \State $*ll\_lookups[i] \gets add\_lookup\_items(bf\_poss[i])$ \algorithmiccomment{Algorithm~\ref{algo:addllLookup}}
  \EndFor

  \\
  \State //add query to query manager link-list  
  \State $add\_query\_item(query\_id, block\_id, **ll\_lookups)$ \algorithmiccomment{Algorithm~\ref{algo:addllQuery}}

\EndFunction
\end{algorithmic}
\end{algorithm}

%%%%%%%%%%%%%%%%%%%%%%%%%%%%%%%%%%%%%%%%
\begin{algorithm}
\caption{Adding item in query link-list}
\label{algo:addllQuery}
\begin{algorithmic}
\Function{add\_query\_item}{$query\_id, block\_id, **ll\_lookups$}
  
  \State $ptr \gets $ allocate new node
  \State $ptr.block\_id \gets block\_id$
  \\
  \For{each *lookups[i]}
    \State $ptr.bitmask[i] \gets $ generate bitmask from $(*ll\_lookups[i]).pos$
    \State $ptr.ptr\_lookup[i] \gets *ll\_lookups[i]$
  \EndFor
  \\
  \State Add to the end of the link-list
  \State \Return $ptr$
\EndFunction
\end{algorithmic}
\end{algorithm}

%%%%%%%%%%%%%%%%%%%%%%%%%%%%%%%%%%%%%%%%
\begin{algorithm}
\caption{Adding item in lookup link-list}
\label{algo:addllLookup}
\begin{algorithmic}
\Function{add\_lookup\_items}{$pos$}

    \State /* Lookup link-list is sorted according to the lookup position */
    \State $ptr \gets $ allocate new node
    \State $ptr.pos \gets pos$
    \State $ptr.value \gets 0$
    \State $ptr.processed \gets 0$

    \\
    \State Find a suitable position in the lookup link-list

    \If{item $i$ exists with the same $pos$ value as $ptr$}
      \If{$i.processed$}
        \State Add $ptr$ next to the item
      \Else
        \State $i.associated \gets i.associated + 1$ 
        \State // associate : no. of query item associated with the lookup item
        \State add a dummy item in the end
        \State release $ptr$
        \State \Return i
      \EndIf
    \Else
      \State Add to the suitable position      
    \EndIf
    \State $ptr.associated \gets 1$

    \If{$ ptr.pos < (*cur\_lookup\_ptr).pos$}
      \State /* $ptr$ must be processed before $cur\_lookup\_ptr$ */
      \State $cur\_lookup\_ptr \gets ptr$
    \EndIf

    \State \Return $ptr$
\EndFunction
\end{algorithmic}
\end{algorithm}

%%%%%%%%%%%%%%%%%%%%%%%%%%%%%%%%%%%%%%%%
\begin{algorithm}
\caption{Bloom filter search}
\label{algo:bfsearch}
\begin{algorithmic}
\Function{process\_block}{$query\_data, block\_id$}
    \\

    %\algorithmiccomment{Process queries that arrived in this block}
   
    \State Extract queries from $query\_data$ (see Algo~\ref{algo:extractQuery})
    \If {$block\_id$ equals $0$}
        \State $dict\_pos \gets 0$ \hskip3em //byte position in dictionary
        \State // $lookup\_tail$ (dummy item) is never processed so
        \State $cur\_lookup\_ptr \gets lookup\_head$ 
    \EndIf
    \\
    \State $mem\_pos \gets $ starting address of the mapped memory
    \State $mem\_end\_pos \gets $ ending address of the mapped memory
    %\State $ptr\_lookup \gets $ current item in the lookup link-list
    \State $cmp\_pos \gets (*cur\_lookup\_ptr).pos $
    \\ 
    \While{$mem\_pos < mem\_end\_pos$}
      \State $(*cur\_lookup\_ptr).value \gets *mem\_pos$
      \\
      \If {$cmp\_pos$ equals $ dict\_pos$}
        \State $(*cur\_lookup\_ptr).processed \gets 1$
      \Else       
        \State $(*cur\_lookup\_ptr).processed \gets 0$
      \EndIf
      \\
      \State // Some lookup items may be processed in prev. round
      \State // but not reached its complete carousel cycle to be collected
      \While{$(*cur\_lookup\_ptr).processed$ equals $1$}
        
        \State $cur\_lookup\_ptr \gets (*cur\_lookup\_ptr).next$
      \EndWhile
      \\
      \State $cmp\_pos \gets (*cur\_lookup\_ptr).pos $
      \State $dict\_pos \gets dict\_pos + 1$
      \State $mem\_pos \gets mem\_pos + 1$
    \EndWhile
    \\
    \State $response \gets $ collect processed responses
    \State \Return $response$
\EndFunction
\end{algorithmic}
\end{algorithm}

\begin{algorithm}
\caption{Bloom filter search ball and bin method}
\begin{algorithmic}
\Function{process\_block}{$queries, block\_id$}

    %\State add\_queries($queries$);
    \\
    \State Extract queries from $query\_data$ (see Algo~\ref{algo:extractQuery})
    \If {$block\_id$ equals $0$}
        \State $dict\_pos \gets 0$ \hskip3em //byte position in dictionary
        \State // $lookup\_tail$ (dummy item) is never processed so
        \State $cur\_lookup\_ptr \gets lookup\_head$ 
    \EndIf
    \\
    \State $mem\_pos \gets $ starting address of the mapped memory
    \State $mem\_end\_pos \gets $ ending address of the mapped memory
    \\ 
    \While{$mem\_pos < mem\_end\_pos$}
      \State $cmp\_pos \gets (*cur\_lookup\_ptr).pos $
      
      \\
      \While{$(dict\_pos < cmp\_pos \leq (dict\_pos + PG\_SIZE))$} 
        \State $lookup\_pos \gets (cmp\_pos - dict\_pos)$
        \State $ptr\_lookup {\rightarrow} value \gets *(mem\_pos + lookup\_pos)$
        \State $ptr\_lookup {\rightarrow} processed \gets 1$
        \State $ptr\_lookup \gets ptr\_lookup {\rightarrow} next$
        \State $cmp\_pos \gets (*cur\_lookup\_ptr).pos  $
        \State $hits\_in\_pg \gets hits\_in\_pg + 1$
      \EndWhile
      \\
      \While{$hits\_in\_pg < EXP\_HITS\_IN\_PG$} 
        \State $rand\_pos \gets Random(0 \cdots PG\_SIZE)$
        \State $ptr\_lookup {\rightarrow} value \gets *(mem\_pos + rand\_pos)$
        \State $hits\_in\_pg \gets hits\_in\_pg + 1$
      \EndWhile
      \\
      \State $dict\_pos \gets dict\_pos + PG\_SIZE$
      \State $mem\_pos \gets mem\_pos + PG\_SIZE$  
    \EndWhile
    \\
    \State $response \gets $ collect processed responses
    \State \Return $response$
\EndFunction

\end{algorithmic}
\end{algorithm}

\begin{algorithm}
\caption{Collect process queries}
\begin{algorithmic}
\Function{collect\_processed\_query}{$block\_id$}
  \State 
  \State $ptr\_query \gets $ the first item in the query manager link-list

  \For{each $ptr\_query$ that is equal to $block\_id$}
    \\
    \State $ptr \gets ptr\_query$
    \For{each $ptr{\rightarrow}ptr\_lookup$}
      \If {$ptr{\rightarrow}ptr\_lookup[i]{\rightarrow}value$ AND $ptr{\rightarrow}bitmask[i]$}
        \State $count \gets count + 1$
      \EndIf 
      \State $ptr{\rightarrow}ptr\_lookup[i]{\rightarrow}n\_associated ~-= 1$
      \If {$(ptr{\rightarrow}ptr\_lookup[i]{\rightarrow}n\_associated == 0) $}
        \State remove $ptr{\rightarrow}ptr\_lookup[i]$ from lookup link-list
      \Else
        \State remove a dummy item from lookup link-list
      \EndIf     
    \EndFor

    \If {$count == BF\_POSS $}
      \State $results || \gets ptr{\rightarrow}id || 1$
    \Else
      \State $results || \gets ptr{\rightarrow}id || 0$
    \EndIf
    \\ 
    \State $ptr\_query \gets ptr\_query{\rightarrow}next$
    \State remove $ptr$ from query link-list
  \EndFor

  \State \Return $results$
\EndFunction
\end{algorithmic}
\end{algorithm}
