# Supplementary material for: Towards Fairness of Cryptocurrency Payments
Source: arXiv:1609.07256 source file (2016-12-01)
Supplement: Supplementary file 2 [file appendix_opt.tex]

%!TEX root = ../submission.tex
\appendix
\section{Code optimization}
\label{sec:appendA}

%Disassembling machine-level instruction  mnemonics showed that naively implementing algorithms from Section~\ref{sec:dictRep} does not ensure equal number of operations on every item in $Y$.
Implementing algorithms from Section~\ref{sec:dictRep} naively does not ensure that the TA performs equal number of operations on every item in $Y$ at machine-level instructions.
For example, in Algorithm~\ref{algo:cuckoo}, \texttt{R} can be an \texttt{unsigned char} array and \texttt{dummy\_byte} an \texttt{unsigned char} variable. The compiler uses different sets of instructions to copy values of $Y$ on to them causing unequal number of machine-level instructions at the conditional clauses (\texttt{if} and \texttt{else}).
Similary, the compiler removes or optimizes the dummy operation (e.g. \texttt{dummy\_int ++}) if they are not used elsewhere in the code. It also removes dummy conditional clauses that are unreachable~/~unnecessary.

We tailored our implementation to achieve a balanced set of instructions for the conditional clauses while processing the carousel. Figure~\ref{Ccode} depicts a section of the carousel processing code for Cuckoo hash method that produces equal number of operations on every item in $Y$ at machine-level instructions. 
Figure~\ref{ASMcode} shows the disassembled machine-level instructions mnemonics for the same code segment.
For similicity the code segment shown in the figure is for processing 16-bit ($\varepsilon=14$) items in $Y$.

In Figure~\ref{Ccode}, \texttt{ptr\_query\_rep} represents the pointer to $S$. 
We use the same variable to represent the dictionary positions as well as store the value of the corresponding position. We implemented the code to operate on 32-bit values. The variables \texttt{ptr\_query\_rep}, \texttt{ptr\_chunk} and \texttt{ptr\_chunk\_end} are defined as \texttt{unsigned int*}. Similarly \texttt{dummy\_pos} is an array of type \texttt{unsigned int}.

%We represent the query as 10 positions of bytes within $Y$ and sort them according to their positions.

% The TA computes the bloom-filter positions of each querie and identifies the locations of the bytes where the bloom-filter positions are mapped.
% The TA arranges the byte locations of bloom-filter position in a sorted order and used it as query representation.
% During carousel, 

% However, in our implementation we use byte position with a bit mask to correctly identify the bloom filter positions.
% We calculated the bloom filter positions using lookup hash function with 10 different seeds.
% The query representations are arranged according to their byte positions. 
% TA picks the query representation with the smallest value and compares it against the dictionary positions.

\begin{figure}[h]
\centering
\begin{lstlisting}[frame=single]
  // ptr_chunk: pointer to the 
  // begining of Y chunk

  // ptr_chunk: pointer to the
  // end Y chunk

  // y_pos: current position
  // in Y

  // ptr_query_rep: pointer to S

  // dummy_pos: dummy array of size 255

 while(ptr_chunk < ptr_chunk_end)
 {
    if(y_pos == *ptr_query_rep)
    {
      *ptr_query_rep = *ptr_chunk;
      ptr_query_rep++;
    } else {
      dummy_pos[(uint8_t)*ptr_chunk] = \
      *ptr_chunk;    
    }
    y_pos ++;
    ptr_chunk = ptr_chunk + 1;
}
\end{lstlisting}
\caption{Kinibi TA code for Cuckoo-on-a-Carousel processing}
\label{Ccode}
\end{figure}

\begin{figure}[h]
\begin{lstlisting}[frame=single]
70e:  1b61       subs    r1, r4, r5
710:  4439       add     r1, r7
712:  f5b1 1f40  cmp.w   r1, #3145728  ; 0x300000
716:  f1c5 0200  rsb r2, r5, #0
71a:  d20a       bcs.n   732 <tlMain+0x1b4>
71c:  6819       ldr r1, [r3, #0]
71e:  4422       add r2, r4
720:  5dd2       ldrb    r2, [r2, r7]
722:  428f       cmp r7, r1
724:  bf0c       ite  eq
726:  f843 2b04  streq.w r2, [r3], #4
72a:  f84a 2022  strne.w r2, [sl, r2, lsl #2]
72e:  3701       adds  r7, #1
730:  e7ed       b.n   70e <tlMain+0x190>
\end{lstlisting}
\caption{Disassembled machine instructions mnemonics for Cuckoo-on-a-Carousel processing}
\label{ASMcode}
\end{figure}
