# Supplementary material for: Towards Fairness of Cryptocurrency Payments
Source: arXiv:1609.07256 source file (2016-12-01)
Supplement: Supplementary file 3 [file appendix.tex]

%!TEX root = ../submission.tex
\section*{Appendix A: Notation Table}
\label{sec:appendA}
